# Supplementary material for: Video Prediction via Example Guidance
Source: arXiv:2007.01738 source file (2020-07-03)
Supplement: Supplementary file 1 [file supp.pdf]

# Supplementary Material of Video Prediction via Example Guidance \*

## 1. Implementation Details

### 1.1. Disentangling Model $\phi_{dse}$

Disentangling mode  $\phi_{dse}$  generally follows the autoencoder architecture. As presented in the main manuscript, the detailed implementation of disentangling model  $\phi_{dse}$  varies accordingly on different datasets. More specifically, on MovingMnist (Srivastava et al., 2015) and Bair RobotPush (Ebert et al., 2017) dataset we build  $\phi_{dse}$  based on SVG (Denton & Fergus, 2018), while on PennAction (Zhang et al., 2013) dataset  $\phi_{dse}$  is identical to the work of Kim et al. (2019). In the following paragraph we present detailed implementation details on MovingMnist (Srivastava et al., 2015) and Bair RobotPush (Ebert et al., 2017) dataset. Please refer to Kim et al. (2019) for training and network details on PennAction (Zhang et al., 2013) dataset.

**On MovingMnist (Srivastava et al., 2015) Dataset.** The encoder part consists of 5 convolutional layers with kernel size 3 and stride 2. The output channel of all 5 layers are 16 / 32 / 64 / 128 / 128 respectively. Batch-normalization layer (Ioffe & Szegedy, 2015) is applied after each convolutional layer. The activation layer is LeakyReLU (Xu et al., 2015) with leaky rate 0.2. Note that the final activation layer is replaced with Tanh function. The decoder part consists of 5 de-convolutional layers with kernel size 3 and stride 2. The output channel of all 5 layers are 128 / 64 / 32 / 16 / 1 respectively (digit is gray scale image). Batch-normalization (Ioffe & Szegedy, 2015) along with LeakyReLU (Xu et al., 2015) (leaky rate 0.2) layers are applied after convolutional layers, where the activation function of outputs is replaced with sigmoid.

**On RobotPush (Ebert et al., 2017) Dataset.** The architecture on this dataset is inspired from vgg net (Simonyan & Zisserman, 2015) and consists of 5 blocks. Each of the first 2 blocks contains 2 convolutional layers with kernel size 3 and stride 1. That of the middle 2 blocks contains 3 convolutional layers with same kernel size and stride. The outputs of first 4 blocks are processed by a maxpooling layer with kernel size 2 and stride 2. The output channels of all 5 blocks are 64 / 128 / 256 / 512 / 512 respectively. Batch-normalization layer (Ioffe & Szegedy, 2015) is applied after each convolutional layer. The activation layer is LeakyReLU (Xu et al., 2015) with leaky rate 0.2. The decoder part consists of 5 de-convolutional blocks with kernel size 3 and stride 2. The architecture of each block is a mirrored version of

the encoder. The maxpooling layer is replaced with nearest-neighbour upsampling layer. Batch-normalization (Ioffe & Szegedy, 2015) along with LeakyReLU (Xu et al., 2015) (leaky rate 0.2) layers are applied after all convolutional layers, where the activation function of outputs is replaced with sigmoid.

**Skip Connection.** As mentioned in the main manuscript, skip connection is used between the encoder and decoder part. More specifically, the outputs of first 4 layers of encoder (on MovingMnist (Srivastava et al., 2015) dataset) or first 4 blocks (on RobotPush (Ebert et al., 2017) dataset) are feed as skip connections to the decoder part.

### 1.2. Prediction Model $\phi_{pre}, \phi_{qz}$

Both  $\phi_{pre}$  and  $\phi_{qz}$  are two-layer LSTM (Hochreiter & Schmidhuber, 1997) networks. For  $\phi_{pre}$ , as mentioned in Eqn. 9 in the main manuscript, the input consists of three components, i.e., current feature  $\hat{\mathbf{f}}_{i,t}$ , random noise  $\mathbf{z}_{i,t}$  and example guidance  $\mathbf{f}_{i:t+1}^\Omega$  respectively. Example guidance  $\mathbf{f}_{i:t+1}^\Omega$  is processed with first-order temporal difference and then feed into one fully connected layer which fuses  $N$  examples into single one. Therefore the dimensions of three components on three datasets are 128 / 20 / 128 (MovingMnist (Srivastava et al., 2015) dataset); 512 / 20 / 512 (RobotPush (Ebert et al., 2017) dataset); 89 / 10 / 89 (PennAction (Zhang et al., 2013) dataset). The input dimension of feature on PennAction (Zhang et al., 2013) dataset is defined by  $40 \times 2 + 9 = 89$ , where 40 is the 2D key-point number and 9 refers to the number of action classes. All three input components are fused by a fully connected layer to 1024 dimension. For  $\phi_{pre}$ , the input and output dimension is thus defined by  $\mathbf{f}_t^\Omega$  and  $\mathbf{z}_{i,t}$  on corresponding datasets respectively.

**Training details.** Note that the disentangling model requires training process on MovingMnist (Srivastava et al., 2015) and RobotPush (Ebert et al., 2017) datasets. This part is implemented with Pytorch (Paszke et al., 2019) framework. Adam optimizer (Kingma & Ba, 2015) is applied with learning rate  $\eta = 1e^{-4}$ ,  $\alpha = 0.5$  and  $\beta = 0.9$ . The weight decay rate is  $1e^{-5}$ . On both MovingMnist (Srivastava et al., 2015) and RobotPush (Ebert et al., 2017) datasets, the model is trained with 50 epoches with stepped learning rate decay at 20th epoch (0.1) and 40th epoch (0.01) respectively. The prediction model is implemented with Pytorch (Paszke et al., 2019) framework on MovingMnist (Srivastava et al., 2015) and RobotPush (Ebert et al., 2017) datasets, while

\*Project page: <https://sites.google.com/view/vpeg-sup/home>

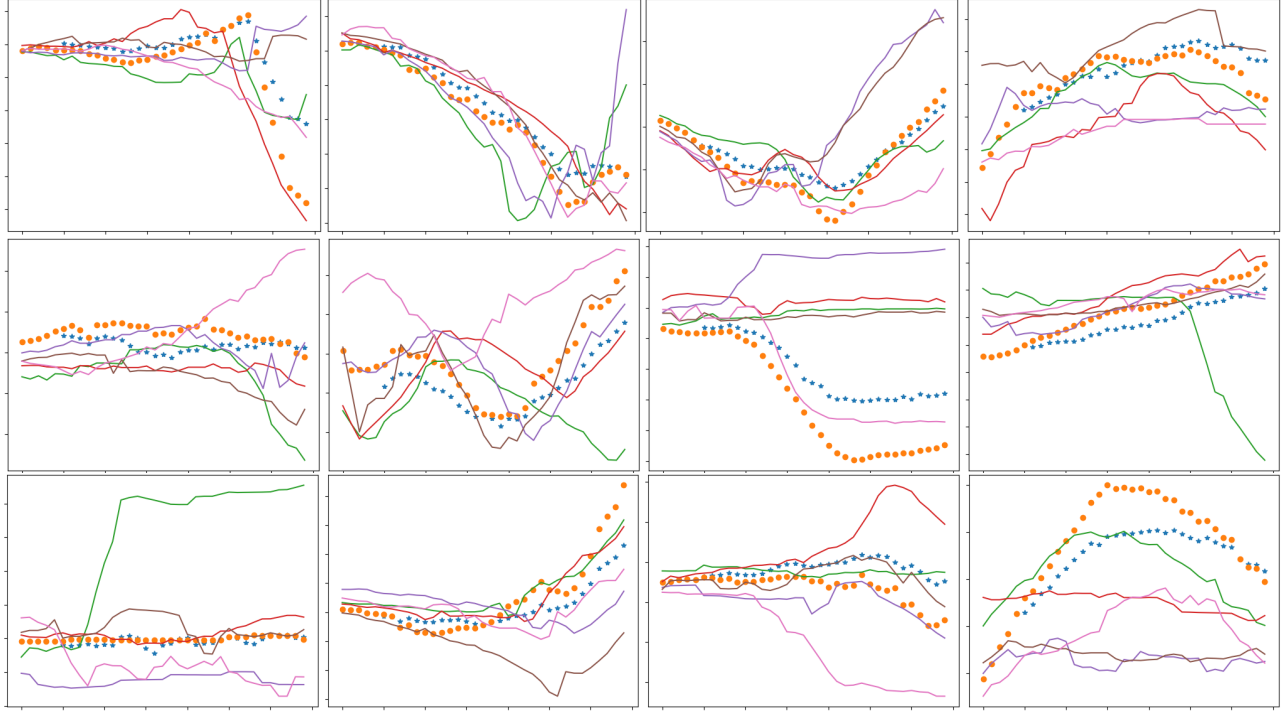

Figure 1. Visualization of retrieved examples on PennAction (Zhang et al., 2013) dataset. For all sub-figures, the X-axis stands for time step and Y-axis refers to the value corresponding to one dimension of learned motion feature. For notation, the 5 solid lines are retrieved example sequence and blue star refers to predicted sequence. Orange-dot line is the ground truth.

tensorflow (Abadi et al., 2015) on PennAction (Zhang et al., 2013) dataset. For all datasets, Adam optimizer (Kingma & Ba, 2015) is applied with learning rate  $\eta = 3e^{-5}$ ,  $\alpha = 0.9$  and  $\beta = 0.999$ . The weight decay rate is  $1e^{-4}$ . The prediction model is trained with 300 epoches with stepped learning rate decay at 100th epoch (0.1) and 200th epoch (0.01) respectively.

## 2. Visualization of Retrieved Examples

As illustrated in Fig. 1, we present more retrieved examples on PennAction (Zhang et al., 2013) dataset. Please refer to the caption for detailed definition of the figure. Here we emphasise two main observations mentioned in main manuscript: (1) The examples generally multi-modal distributed, which implies the difficulty on the optimization side by a variational inference method. (2) The input sequence generally falls into one motion pattern of retrieved examples, which confirms the key insight of our work. **We provide more predicted results on this anonymous website<sup>1</sup>. Please refer to it.**

<sup>1</sup><https://sites.google.com/view/vpeg-sup/home>

## 3. MovingMnist Prediction

### 3.1. Visualization of Deterministic Prediction

As shown in Fig. 2, we present a typical result evaluated under deterministic MovingMnist (Srivastava et al., 2015) prediction. Please refer to the caption for detailed experiment setting. As highlighted by red box in Fig. 2, SVG (Denton & Fergus, 2018) fails to give accurate prediction even calculating the best of 20 random sequences. In contrast to SVG (Denton & Fergus, 2018), guided by retrieved examples our model is able to synthesise plausible future frames. DFN (Shi et al., 2015) also gives relative accurate prediction under deterministic setting, but it is infeasible to handle stochastic prediction properly. Details are presented in following paragraph.

### 3.2. Visualization of Stochastic Prediction

As shown in Fig. 3, we present a typical result evaluated under stochastic MovingMnist (Srivastava et al., 2015) prediction. Please refer to the caption for detailed experiment setting. As highlighted by red box in Fig. 2, the prediction results of DFN (Denton & Fergus, 2018) demonstrate severe image quality degeneration effect, which mainly results from the incapability of capturing uncertainty of future

|              |   |   |   |   |   |   |   |   |   |   |   |   |   |   |   |
|--------------|---|---|---|---|---|---|---|---|---|---|---|---|---|---|---|
| Ground Truth | 3 | 3 | 3 | 3 | 3 | 3 | 3 | 3 | 3 | 3 | 3 | 3 | 3 | 3 | 3 |
| Example      | 4 | 4 | 4 | 4 | 4 | 4 | 4 | 4 | 4 | 4 | 4 | 4 | 4 | 4 | 4 |
| Ours         | 3 | 3 | 3 | 3 | 3 | 3 | 3 | 3 | 3 | 3 | 3 | 3 | 3 | 3 | 3 |
| SVG-LP       | 3 | 3 | 3 | 3 | 3 | 3 | 3 | 3 | 3 | 3 | 3 | 3 | 3 | 3 | 3 |
| DFN          | 3 | 3 | 3 | 3 | 3 | 3 | 3 | 3 | 3 | 3 | 3 | 3 | 3 | 3 | 3 |

Figure 2. Demonstration of predicted results on MovingMnist (Srivastava et al., 2015) dataset under deterministic setting. Rows from top to bottom refer to ground truth, retrieved example, predicted results of our model, SVG (Denton & Fergus, 2018) and DFN (Shi et al., 2015) respectively. Sub-sequences are highlighted with red box for better evaluation.

|              |   |   |   |   |   |   |   |   |   |   |   |   |   |   |   |
|--------------|---|---|---|---|---|---|---|---|---|---|---|---|---|---|---|
| Ground Truth | 5 | 5 | 5 | 5 | 5 | 5 | 5 | 5 | 5 | 5 | 5 | 5 | 5 | 5 | 5 |
| Example      | 2 | 2 | 2 | 2 | 2 | 2 | 2 | 2 | 2 | 2 | 2 | 2 | 2 | 2 | 2 |
| Ours         | 5 | 5 | 5 | 5 | 5 | 5 | 5 | 5 | 5 | 5 | 5 | 5 | 5 | 5 | 5 |
| SVG-LP       | 5 | 5 | 5 | 5 | 5 | 5 | 5 | 5 | 5 | 5 | 5 | 5 | 5 | 5 | 5 |
| DFN          | 5 | 5 | 5 | 5 | 5 | 5 | 5 | 5 | 5 | 5 | 5 | 5 | 5 | 5 | 5 |

Figure 3. Demonstration of predicted results on MovingMnist (Srivastava et al., 2015) dataset under stochastic setting. Rows from top to bottom refer to ground truth, retrieved example, predicted results of our model, SVG (Denton & Fergus, 2018) and DFN (Shi et al., 2015) respectively. The best one of 20 random samples (in terms of PSNR) is presented. Sub-sequences are highlighted with red box for better evaluation.

states. In contrast to DFN (Denton & Fergus, 2018), guided by retrieved examples our model is able to synthesise plausible future frames, i.e., bouncing back when hitting the boundary meanwhile generally following the moving trajectory of ground truth sequence. SVG (Shi et al., 2015) gives more rational prediction than DFN (Denton & Fergus, 2018), but it is infeasible to learn the underlying motion pattern accurately.

## 4. Robot Arm Prediction

### 4.1. Prediction Accuracy Comparison

To evaluate the prediction accuracy on RobotPush (Ebert et al., 2017) dataset, we compare our model with SVG (Denton & Fergus, 2018) and SV2P (Babaeizadeh et al., 2018). As shown in Fig. 4. please refer to the caption for detailed

experiment setting. Prediction error is highlighted with red box for better evaluation, which demonstrates a general robot arm movements from center to right side. Retrieved example matches well with the ground truth motion, which effectively facilitates the prediction model capturing multi-modal patterns more reliably. **We provide more predicted results on this anonymous website<sup>2</sup>. Please refer to it.**

### 4.2. Prediction Diversity Visualization

To evaluate the prediction diversity on RobotPush (Ebert et al., 2017) dataset, we present randomly sampled sequences in Fig. 5. Please refer to the caption for detailed experiment setting. We can notice that the prediction model with example guidance is able to synthesise highly diverse

<sup>2</sup><https://sites.google.com/view/vpeg-supply/home>

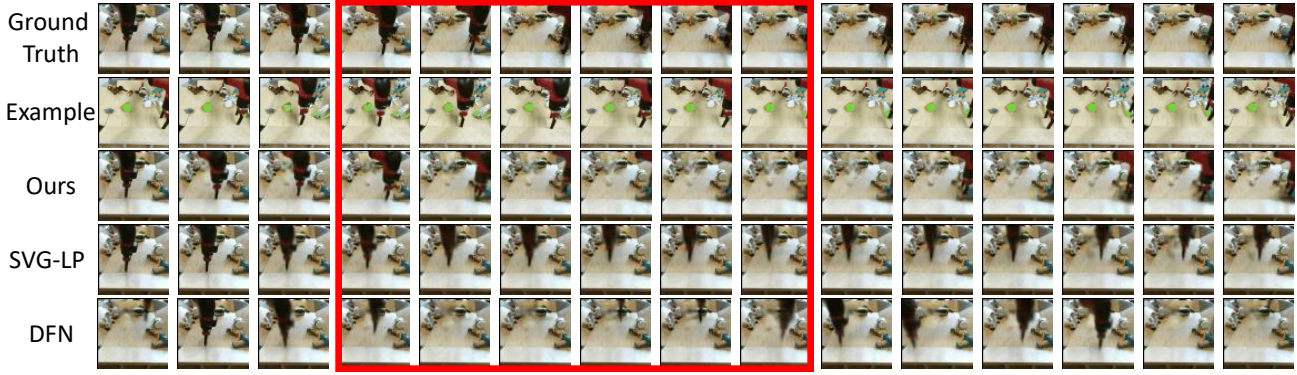

Figure 4. Demonstration of predicted results on RobotPush (Ebert et al., 2017) dataset. Rows from top to bottom refer to ground truth, retrieved example, predicted results of our model, SVG (Denton & Fergus, 2018) and SV2P (Babaeizadeh et al., 2018) respectively. The best one of 20 random samples (in terms of PSNR) is presented. Sub-sequences are highlighted with red box for better evaluation.

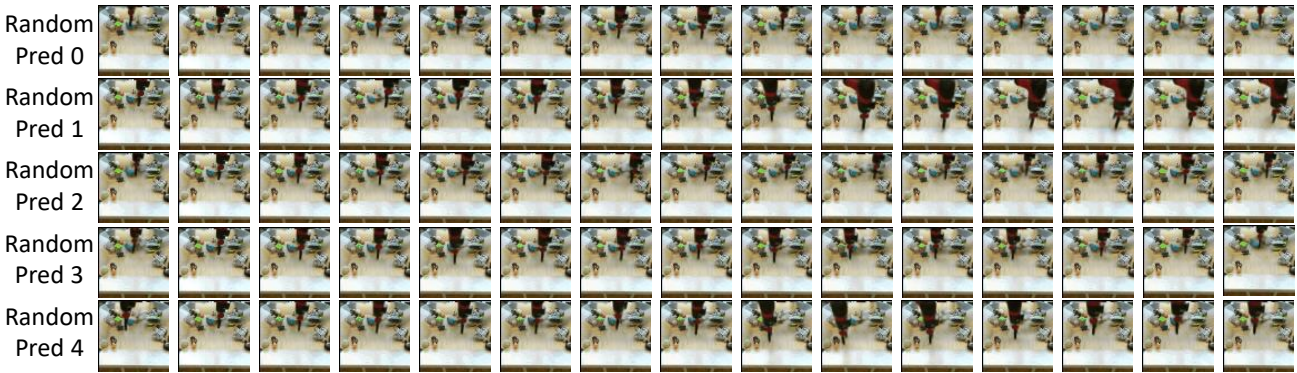

Figure 5. Illustration of randomly predicted results on RobotPush (Ebert et al., 2017) dataset. 5 rows correspond to 5 randomly predicted sequences. We can notice that the trajectories of 5 predicted sequences are highly diverse.

future motion patterns.

## 5. Human Action Prediction

As shown in Fig. 6, we present prediction results on PennAction (Zhang et al., 2013) dataset. Please refer to the caption for corresponding experiment setting. Fig. 6 demonstrates a typical tennis serving action. We highlight the predicted results with red box for better comparison. We can notice that Kim et al. (2019) gives irrational prediction, i.e., the wrong tennis serving direction (please note the difference of leg movements between ground truth and the results of Kim et al. (2019)). In contrast to Kim et al. (2019), our model makes it to synthesise plausible motion (please note the body leaning direction and leg movements), which is mainly facilitated by the guidance of retrieved example (last row in Fig. 6). **We provide more predicted results on this**

anonymous website<sup>3</sup>. Please refer to it.

## 6. Training under Variational Inference

We present predicted results (Fig. 7) trained under variational inference as described in Sec. 3.2.2 of the main manuscript. Please refer to the caption of Fig. 7 for detailed experimental setting. We can notice that the prediction model is infeasible to synthesise rational results. Both best predicted sequence and random sampled one are severely distorted. The digit 1 is not properly preserved during the whole prediction procedure. This mainly results from that the assumption of prior distribution in variational inference is Gaussian distribution, which is conflict with multi-modal distributed examples. More specifically, during optimization procedure the modelled future dynamics is forced to approximate uni-modal distribution, which finally leads to

<sup>3</sup><https://sites.google.com/view/vpeg-sup/home>

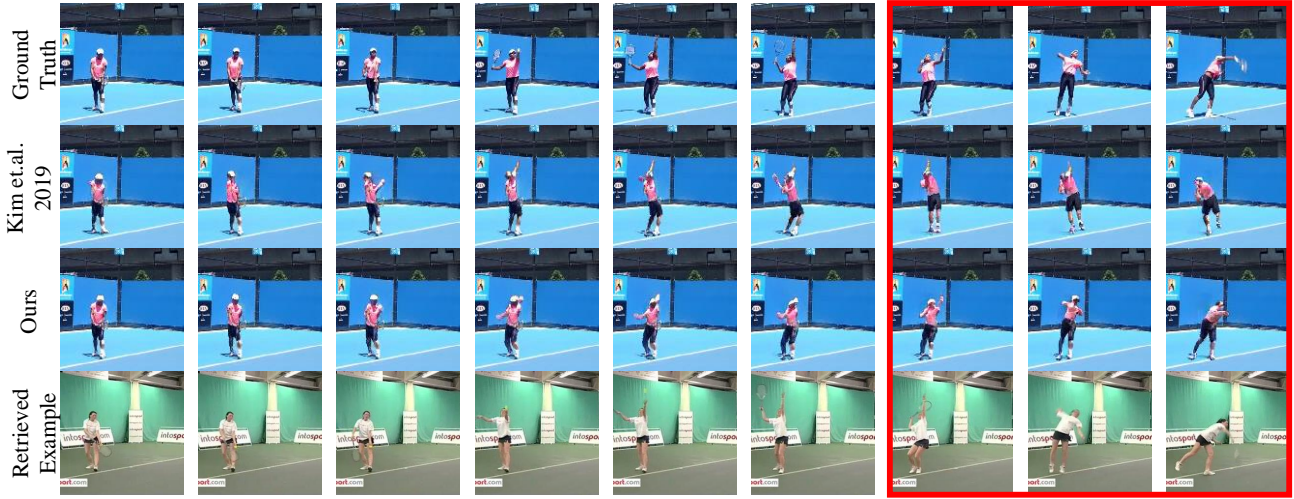

Figure 6. Demonstration of predicted results on PennAction (Zhang et al., 2013) dataset. Rows from top to bottom refer to ground truth, predicted results of Kim et al. (2019), our model and retrieved example respectively. The best one of 20 random samples (in terms of PSNR) is presented. Sub-sequences are highlighted with red box for better evaluation.

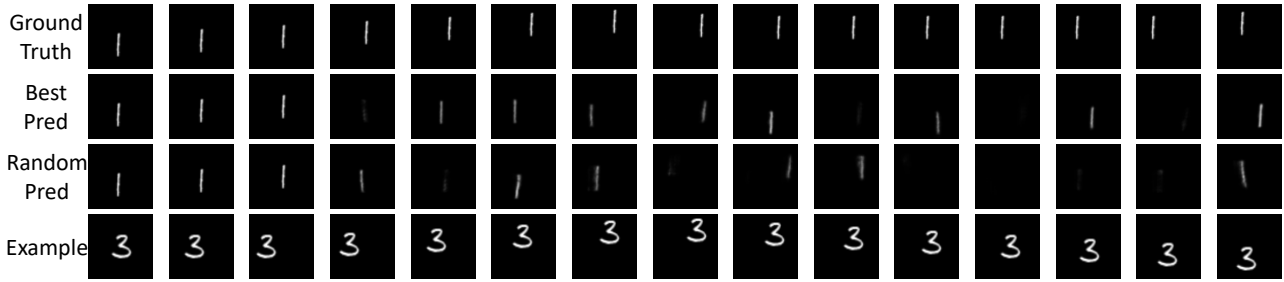

Figure 7. Demonstration of predicted results on MovingMnist (Srivastava et al., 2015) dataset. Note during training the variational inference is used instead of proposed one in our work. Rows from top to bottom refer to ground truth, best predicted result of 20 random samples, one randomly predicted sequences and retrieved example sequence respectively.

sub-optimal results.

## References

- Abadi, M., Agarwal, A., Barham, P., Brevdo, E., Chen, Z., Citro, C., Corrado, G. S., Davis, A., Dean, J., Devin, M., Ghemawat, S., Goodfellow, I., Harp, A., Irving, G., Isard, M., Jia, Y., Jozefowicz, R., Kaiser, L., Kudlur, M., Levenberg, J., Mané, D., Monga, R., Moore, S., Murray, D., Olah, C., Schuster, M., Shlens, J., Steiner, B., Sutskever, I., Talwar, K., Tucker, P., Vanhoucke, V., Vasudevan, V., Viégas, F., Vinyals, O., Warden, P., Wattenberg, M., Wicke, M., Yu, Y., and Zheng, X. TensorFlow: Large-scale machine learning on heterogeneous systems, 2015. URL <https://www.tensorflow.org/>. Software available from tensorflow.org.
- Babaeizadeh, M., Finn, C., Erhan, D., Campbell, R. H., and Levine, S. Stochastic variational video prediction. In *ICLR*, 2018.
- Denton, E. and Fergus, R. Stochastic video generation with a learned prior. In *ICML*, pp. 1182–1191, 2018.
- Ebert, F., Finn, C., Lee, A. X., and Levine, S. Self-supervised visual planning with temporal skip connections. In *CoRL*, pp. 344–356, 2017.
- Hochreiter, S. and Schmidhuber, J. Long short-term memory. *Neural Computation*, 9(8):1735–1780, 1997.
- Ioffe, S. and Szegedy, C. Batch normalization: Accelerating deep network training by reducing internal covariate shift. In *ICML*, pp. 448–456, 2015.

- 
- Kim, Y., Nam, S., Cho, I., and Kim, S. J. Unsupervised  
keypoint learning for guiding class-conditional video pre-  
diction. In *NeurIPS*, pp. 3809–3819, 2019.
- Kingma, D. P. and Ba, J. Adam: A method for stochastic  
optimization. In *ICLR*, 2015.
- Paszke, A., Gross, S., Massa, F., Lerer, A., Bradbury, J.,  
Chanan, G., Killeen, T., Lin, Z., Gimelshein, N., Antiga,  
L., Desmaison, A., Kopf, A., Yang, E., DeVito, Z., Raison,  
M., Tejani, A., Chilamkurthy, S., Steiner, B., Fang, L.,  
Bai, J., and Chintala, S. Pytorch: An imperative style,  
high-performance deep learning library. In *NeurIPS*, pp.  
8024–8035. 2019.
- Shi, X., Chen, Z., Wang, H., Yeung, D., Wong, W., and Woo,  
W. Convolutional LSTM network: A machine learning  
approach for precipitation nowcasting. In *NeurIPS*, pp.  
802–810, 2015.
- Simonyan, K. and Zisserman, A. Very deep convolutional  
networks for large-scale image recognition. In *ICLR*,  
2015.
- Srivastava, N., Mansimov, E., and Salakhutdinov, R. Unsu-  
pervised learning of video representations using lstms. In  
*ICML*, pp. 843–852, 2015.
- Xu, B., Wang, N., Chen, T., and Li, M. Empirical evaluation  
of rectified activations in convolutional network. *CoRR*,  
abs/1505.00853, 2015.
- Zhang, W., Zhu, M., and Derpanis, K. G. From actemes to  
action: A strongly-supervised representation for detailed  
action understanding. In *ICCV*, pp. 2248–2255, 2013.
